# Supplementary material for: BotNet: A Simulator for Studying the Effects of Accurate Communication Models on Multi-agent and Swarm Control
Source: arXiv:2108.13606 source file (2021-08-31)
Supplement: Supplementary file 1 [file _appendics.tex]

% \section*{Appendix}

% \subsection{Flocking with Minimal Scheduling Function}
% The 6TiSCH simulator includes a minimal schedule function by default, which is designed for stationary nodes.
% These experiments are a supplement to those shown in \sect{sec:exp}, specifically \fig{fig:flock1}.

% \begin{figure}[t]
%     \centering
%     \includegraphics[width=.9\linewidth]{figures/MSF_flock.pdf}
%     \caption{
%     Median and standard deviation flocking velocity for different potential control connectivity radii (10 trials per configuration, 10 agents per trial, MSF). 
%     Average velocities close to zero generally indicate that the flock fails to follow the leader agent. 
%     The results show that using more realistic propagation models in the networking simulation stack sets bounds on the potential control flocking radius; at higher radii, agents lose connection from the leader and potentially their neighbors (depending on collision radius).
%     }
%     \label{fig:flock_msf}
% \end{figure}
